# Supplementary material for: Individual correlations in ensemble density-functional theory: State-driven/density-driven decompositions without additional Kohn-Sham systems
Source: arXiv:2001.08605 source file (2020-05-27)
Supplement: Supplementary file 1 [file supp_mat_for_revision.pdf]

# Supplementary material to the manuscript “Individual correlations in ensemble density-functional theory: State-driven/density-driven decompositions without additional Kohn–Sham systems”

Emmanuel Fromager<sup>1</sup>

<sup>1</sup>*Laboratoire de Chimie Quantique,  
Institut de Chimie, CNRS / Université de Strasbourg,  
4 rue Blaise Pascal, F-67000 Strasbourg, France*

Additional derivations, comments on the exact theory, and a detailed application of the two state-driven/density-driven decompositions to the weakly asymmetric and strongly correlated Hubbard dimer are provided in the present supplemental material.

## I. EXACT THEORY: COMPLEMENTS AND COMMENTS

### A. Static ensemble linear response equations

In the following we denote  $i$  (or  $j$ ) the orbitals that are occupied in the ensemble, i.e. those that fulfill  $\sum_{K=0}^M \mathbf{w}_K \theta_i^K > 0$ . Unoccupied orbitals will be denoted as  $a$ . According to the ensemble KS equations and first-order perturbation theory, the response of the occupied KS orbitals reads

$$\frac{\partial \varphi_i^{\mathbf{w}}(\mathbf{r})}{\partial \mathbf{w}_I} = \sum_a \frac{\langle \varphi_a^{\mathbf{w}} | \hat{\mathcal{V}}_{\text{Hxc}, \mathbf{w}_I}^{\mathbf{w}} | \varphi_i^{\mathbf{w}} \rangle}{\varepsilon_i^{\mathbf{w}} - \varepsilon_a^{\mathbf{w}}} \varphi_a^{\mathbf{w}}(\mathbf{r}), \quad (1)$$

where the local multiplicative perturbation operator  $\hat{\mathcal{V}}_{\text{Hxc}, \mathbf{w}_I}^{\mathbf{w}} \equiv \mathcal{V}_{\text{Hxc}, \mathbf{w}_I}^{\mathbf{w}}(\mathbf{r}) \times$  is defined as follows:

$$\begin{aligned} \mathcal{V}_{\text{Hxc}, \mathbf{w}_I}^{\mathbf{w}}(\mathbf{r}) &= \frac{d}{d\mathbf{w}_I} \left[ v_{\text{Hxc}}^{\mathbf{w}}[n^{\mathbf{w}}](\mathbf{r}) \right] = \left. \frac{\partial v_{\text{Hxc}}^{\mathbf{w}}[n^{\boldsymbol{\xi}}](\mathbf{r})}{\partial \mathbf{w}_I} \right|_{\boldsymbol{\xi}=\mathbf{w}} \\ &+ \int d\mathbf{r}' \frac{\delta v_{\text{Hxc}}^{\mathbf{w}}[n^{\mathbf{w}}](\mathbf{r})}{\delta n(\mathbf{r}')} \frac{\partial n^{\mathbf{w}}(\mathbf{r}')}{\partial \mathbf{w}_I}. \end{aligned} \quad (2)$$

Note that, like in linear response TD-DFT [1], the perturbation depends on the response of the KS orbitals through the ensemble Hxc kernel contribution [last term on the right-hand side of Eq. (2)]. By expressing the response  $\partial n^{\mathbf{w}}(\mathbf{r})/\partial \mathbf{w}_I$  of the ensemble density in terms of the KS orbitals and their first-order derivatives, we finally obtain the following *static* linear response equation,

$$\begin{aligned} \frac{\partial \varphi_i^{\mathbf{w}}(\mathbf{r})}{\partial \mathbf{w}_I} &= \sum_a \frac{\varphi_a^{\mathbf{w}}(\mathbf{r})}{\varepsilon_i^{\mathbf{w}} - \varepsilon_a^{\mathbf{w}}} \int d\mathbf{r}' \mathcal{V}_{\text{Hxc}, I}^{\mathbf{w}}(\mathbf{r}') \varphi_i^{\mathbf{w}}(\mathbf{r}') \varphi_a^{\mathbf{w}}(\mathbf{r}') \\ &+ 2 \sum_a \sum_j \sum_{K=0}^M \frac{\mathbf{w}_K \theta_j^K \varphi_a^{\mathbf{w}}(\mathbf{r})}{\varepsilon_i^{\mathbf{w}} - \varepsilon_a^{\mathbf{w}}} \int d\mathbf{r}' \int d\mathbf{r}'' \frac{\delta v_{\text{Hxc}}^{\mathbf{w}}[n^{\mathbf{w}}](\mathbf{r}')}{\delta n(\mathbf{r}'')} \\ &\times \varphi_i^{\mathbf{w}}(\mathbf{r}') \varphi_a^{\mathbf{w}}(\mathbf{r}') \varphi_j^{\mathbf{w}}(\mathbf{r}'') \frac{\partial \varphi_j^{\mathbf{w}}(\mathbf{r}'')}{\partial \mathbf{w}_I}, \end{aligned} \quad (3)$$

where

$$\begin{aligned} \mathcal{V}_{\text{Hxc}, I}^{\mathbf{w}}(\mathbf{r}) &= \left. \frac{\partial v_{\text{Hxc}}^{\mathbf{w}}[n^{\boldsymbol{\xi}}](\mathbf{r})}{\partial \mathbf{w}_I} \right|_{\boldsymbol{\xi}=\mathbf{w}} \\ &+ \sum_p (\theta_p^I - \theta_p^0) \int d\mathbf{r}' \frac{\delta v_{\text{Hxc}}^{\mathbf{w}}[n^{\mathbf{w}}](\mathbf{r})}{\delta n(\mathbf{r}')} |\varphi_p^{\mathbf{w}}(\mathbf{r}')|^2 \end{aligned} \quad (4)$$

is what remains from the full perturbation in Eq. (2) when the true densities are approximated by the KS ones. As readily seen from Eq. (3), this part of the perturbation ignites the response of the KS orbitals which should then be updated (*via* the ensemble Hxc kernel contribution) until a self-consistent convergence is reached. Note that, for practical purposes, one should rewrite Eq. (3) as a coupled-perturbed equation, by analogy with Ref. [2]. If the exact ensemble potential and kernel were known, one should ultimately recover the exact linear response, thus leading to the true individual densities. The latter can still be (approximately) described by means of Eq. (3) even if the simple (weight-independent) ground-state functional approximation  $E_{\text{Hxc}}^{\mathbf{w}}[n] \approx E_{\text{Hxc}}[n]$  [3, 4] is employed. Indeed, in the latter case, the first term on the right-hand side of Eq. (4) vanishes but not the second one that involves the conventional ground-state Hxc kernel  $\delta v_{\text{Hxc}}[n](\mathbf{r})/\delta n(\mathbf{r}')$ .

### B. Individual correlation energies versus individual components

The distinction that should be made between the  $J$ th component of the ensemble correlation energy and the  $J$ th individual correlation energy is discussed further in the following. We start from the exact expression, which is obtained from the decomposition of the ensemble cor-

relation energy into components,

$$E_{c,J}^{\mathbf{w}}[n^{\mathbf{w}}] = \mathcal{E}_{c,J}^{\mathbf{w}}[n^{\mathbf{w}}] + \sum_{K=0}^M \mathbf{w}_K \sum_{I=1}^M (\delta_{IJ} - \mathbf{w}_I) \times \frac{\partial}{\partial \mathbf{w}_I} \left( \mathcal{E}_{c,K}^{\mathbf{w}}[n^{\mathbf{w}}] - \mathcal{E}_{c,K}^{\xi}[n^{\xi,\mathbf{w}}] \right) \Big|_{\xi=\mathbf{w}}, \quad (5)$$

where

$$\mathcal{E}_{c,K}^{\mathbf{w}}[n^{\mathbf{w}}] = \langle \Psi_K | \hat{T} + \hat{W}_{ee} | \Psi_K \rangle - \langle \Phi_K^{\mathbf{w}} | \hat{T} + \hat{W}_{ee} | \Phi_K^{\mathbf{w}} \rangle \quad (6)$$

and

$$\mathcal{E}_{c,K}^{\xi}[n^{\xi,\mathbf{w}}] = \left\langle \Psi_K^{\xi}[n^{\xi,\mathbf{w}}] \left| \hat{T} + \hat{W}_{ee} \right| \Psi_K^{\xi}[n^{\xi,\mathbf{w}}] \right\rangle - \langle \Phi_K^{\mathbf{w}} | \hat{T} + \hat{W}_{ee} | \Phi_K^{\mathbf{w}} \rangle. \quad (7)$$

At this point, one should stress that the equality  $\Phi_K^{\xi}[n^{\xi,\mathbf{w}}] = \Phi_K^{\mathbf{w}}$  that holds in the non-interacting case, simply because the density  $n^{\xi,\mathbf{w}}$  is built from the KS wavefunctions  $\{\Phi_J^{\mathbf{w}}\}$ , is *not* necessarily fulfilled in the true interacting case:

$$\Psi_K^{\xi}[n^{\xi,\mathbf{w}}] \neq \Psi_K^{\mathbf{w}}[n^{\mathbf{w}}] = \Psi_K. \quad (8)$$

This is where the situation differs for the exchange and correlation energies. Indeed, at the exchange-only level, individual energies and components match. This is not necessarily the case when correlation is introduced, as readily seen from the following expression:

$$E_{c,J}^{\mathbf{w}}[n^{\mathbf{w}}] = \mathcal{E}_{c,J}^{\mathbf{w}}[n^{\mathbf{w}}] - \sum_{K=0}^M \mathbf{w}_K \sum_{I=1}^M (\delta_{IJ} - \mathbf{w}_I) \times \frac{\partial}{\partial \mathbf{w}_I} \left\langle \Psi_K^{\xi}[n^{\xi,\mathbf{w}}] \left| \hat{T} + \hat{W}_{ee} \right| \Psi_K^{\xi}[n^{\xi,\mathbf{w}}] \right\rangle \Big|_{\xi=\mathbf{w}}. \quad (9)$$

It can be further simplified by introducing individual interacting density-functional energies as follows,

$$\left\langle \Psi_K^{\xi}[n^{\xi,\mathbf{w}}] \left| \hat{T} + \hat{W}_{ee} \right| \Psi_K^{\xi}[n^{\xi,\mathbf{w}}] \right\rangle \quad (10)$$

$$= E_K^{\xi}[n^{\xi,\mathbf{w}}] - \int d\mathbf{r} v^{\xi}[n^{\xi,\mathbf{w}}](\mathbf{r}) n_{\Psi_K^{\xi}[n^{\xi,\mathbf{w}}]}(\mathbf{r}), \quad (11)$$

where  $v^{\xi}[n^{\xi,\mathbf{w}}]|_{\xi=\mathbf{w}} = v_{\text{ext}}$ , and applying the Hellmann–Feynman theorem,

$$\frac{\partial}{\partial \mathbf{w}_I} \left\langle \Psi_K^{\xi}[n^{\xi,\mathbf{w}}] \left| \hat{T} + \hat{W}_{ee} \right| \Psi_K^{\xi}[n^{\xi,\mathbf{w}}] \right\rangle \Big|_{\xi=\mathbf{w}} = - \int d\mathbf{r} v_{\text{ext}}(\mathbf{r}) \frac{\partial n_{\Psi_K^{\xi}[n^{\xi,\mathbf{w}}]}(\mathbf{r})}{\partial \mathbf{w}_I} \Big|_{\xi=\mathbf{w}}, \quad (12)$$

thus leading to

$$E_{c,J}^{\mathbf{w}}[n^{\mathbf{w}}] = \mathcal{E}_{c,J}^{\mathbf{w}}[n^{\mathbf{w}}] + \int d\mathbf{r} v_{\text{ext}}(\mathbf{r}) \times \sum_{K=0}^M \mathbf{w}_K \sum_{I=1}^M (\delta_{IJ} - \mathbf{w}_I) \frac{\partial n_{\Psi_K^{\xi}[n^{\xi,\mathbf{w}}]}(\mathbf{r})}{\partial \mathbf{w}_I} \Big|_{\xi=\mathbf{w}}, \quad (13)$$

which, according to the density constraint

$$\sum_{K=0}^M \xi_K n_{\Psi_K^{\xi}[n^{\xi,\mathbf{w}}]}(\mathbf{r}) = n^{\xi,\mathbf{w}}(\mathbf{r}) = \sum_{K=0}^M \xi_K n_{\Phi_K^{\mathbf{w}}}(\mathbf{r}), \quad (14)$$

is equivalent to

$$E_{c,J}^{\mathbf{w}}[n^{\mathbf{w}}] = \mathcal{E}_{c,J}^{\mathbf{w}}[n^{\mathbf{w}}] + \int d\mathbf{r} v_{\text{ext}}(\mathbf{r}) \times \sum_{K=0}^M \mathbf{w}_K \sum_{I=1}^M (\delta_{IJ} - \mathbf{w}_I) \frac{\partial n_{\Phi_K^{\mathbf{w}}}(\mathbf{r})}{\partial \mathbf{w}_I}. \quad (15)$$

Thus we obtain the simplified (and expected) expression,

$$E_{c,J}^{\mathbf{w}}[n^{\mathbf{w}}] = \mathcal{E}_{c,J}^{\mathbf{w}}[n^{\mathbf{w}}] + \int d\mathbf{r} v_{\text{ext}}(\mathbf{r}) (n_{\Psi_J}(\mathbf{r}) - n_{\Phi_J^{\mathbf{w}}}(\mathbf{r})), \quad (16)$$

where, as readily seen, the individual correlation energy contains a density correction term which does not exist in conventional ground-state DFT.

In the strongly correlated and weakly asymmetric Hubbard dimer, which is discussed in detail in Sec. II, the integral on the right-hand side of Eq. (16) becomes

$$-\Delta v_{\text{ext}}(n_{\Psi_J} - n_{\Phi_J^{\mathbf{w}}}) \stackrel{J=0}{\approx} \frac{\mathbf{w}\eta}{(1-\mathbf{w})} \Delta v_{\text{ext}} = 2U\eta^2 \left( \frac{t}{U} \right)^2 \frac{\mathbf{w}}{(1-\mathbf{w})} \quad (17)$$

and

$$-\Delta v_{\text{ext}}(n_{\Psi_J} - n_{\Phi_J^{\mathbf{w}}}) \stackrel{J=1}{\approx} -\Delta v_{\text{ext}}\eta = -2U\eta^2 \left( \frac{t}{U} \right)^2, \quad (18)$$

where  $\eta = U\Delta v_{\text{ext}}/(2t^2)$ . Since, in the regime under study ( $\eta \ll 1$  and  $t/U \ll 1$ ), correlation energies (per unit of  $U$ ) are zeroth or second order in  $\eta$  [see Sec. II], the difference between individual correlation energies and the components of the ensemble correlation energy will be negligible.

### C. Exact $\overline{\text{SD}}/\overline{\text{DD}}$ density-functional decomposition

The purpose of this section is to show how the *state*-based (so-called  $\overline{\text{SD}}/\overline{\text{DD}}$ ) decomposition of individual correlation energies can be expressed in terms of density-functional *ensemble* quantities. We start from the original expression

$$E_{c,J}^{\mathbf{w},\overline{\text{SD}}}[n^{\mathbf{w}}] := \langle \Psi_J | \hat{T} + \hat{W}_{ee} | \Psi_J \rangle - \langle \Phi_J^{\mathbf{w}} | \hat{T} + \hat{W}_{ee} | \Phi_J^{\mathbf{w}} \rangle - 2 \sum_{I=1}^M (\delta_{IJ} - \mathbf{w}_I) \mathbf{w}_J \left\langle \Phi_J^{\mathbf{w}} \left| \hat{T} + \hat{W}_{ee} \right| \frac{\partial \Phi_J^{\mathbf{w}}}{\partial \mathbf{w}_I} \right\rangle. \quad (19)$$

We recognize in Eq. (19) the *individual* exchange-only GOK energy,

$$f_J^{\mathbf{w}}[n^{\mathbf{w}}] = \langle \Phi_J^{\mathbf{w}} | \hat{T} + \hat{W}_{ee} | \Phi_J^{\mathbf{w}} \rangle, \quad (20)$$

thus leading to the compact expression

$$E_{c,J}^{\mathbf{w},\overline{\text{SD}}}[n^{\mathbf{w}}] = \langle \Psi_J | \hat{T} + \hat{W}_{ee} | \Psi_J \rangle - \bar{f}_J^{\mathbf{w}}[n^{\mathbf{w}}], \quad (21)$$

where

$$\bar{f}_J^{\mathbf{w}}[n^{\mathbf{w}}] = f_J^{\mathbf{w}}[n^{\mathbf{w}}] + \sum_{I=1}^M (\delta_{IJ} - \mathbf{w}_I) \mathbf{w}_J \frac{\partial f_J^{\mathbf{w}}[n^{\mathbf{w}}]}{\partial \mathbf{w}_I}. \quad (22)$$

We now need to relate both terms on the right-hand side of Eq. (21) to density-functional ensemble quantities. Let us start with the second term. Like in the extraction of individual Hx energies, we introduce the two-weight KS ensemble density  $n^{\xi,\mathbf{w}}(\mathbf{r}) = \sum_{I=0}^M \xi_I n_{\Phi_I^{\mathbf{w}}}(\mathbf{r})$ . When inserted into the exchange-only ensemble GOK functional, it allows for an extraction of individual exchange-only energies. Indeed, since

$$f^{\mathbf{w}}[n^{\mathbf{w}}] = \sum_{I=0}^M \mathbf{w}_I f_I^{\mathbf{w}}[n^{\mathbf{w}}] \quad (23)$$

and

$$f^{\xi}[n^{\xi,\mathbf{w}}] = \sum_{I=0}^M \xi_I f_I^{\mathbf{w}}[n^{\mathbf{w}}], \quad (24)$$

it comes

$$\begin{aligned} f_J^{\mathbf{w}}[n^{\mathbf{w}}] &= f^{\mathbf{w}}[n^{\mathbf{w}}] + \sum_{I=1}^M (\delta_{IJ} - \mathbf{w}_I) (f_I^{\mathbf{w}}[n^{\mathbf{w}}] - f_0^{\mathbf{w}}[n^{\mathbf{w}}]) \\ &= f^{\mathbf{w}}[n^{\mathbf{w}}] + \sum_{I=1}^M (\delta_{IJ} - \mathbf{w}_I) \frac{\partial f^{\xi}[n^{\xi,\mathbf{w}}]}{\partial \xi_I}. \end{aligned} \quad (25)$$

Note that, in the exact theory, the derivative on the right-hand side of Eq. (25) is  $\xi$ -independent. It will not be the case anymore when density-functional approximations are employed [see Eq. (68)]. For the sake of generality, the derivative will be taken at  $\xi = \mathbf{w}$ , thus leading to the final expression

$$f_J^{\mathbf{w}}[n^{\mathbf{w}}] = f^{\mathbf{w}}[n^{\mathbf{w}}] + \sum_{I=1}^M (\delta_{IJ} - \mathbf{w}_I) \left. \frac{\partial f^{\xi}[n^{\xi,\mathbf{w}}]}{\partial \xi_I} \right|_{\xi=\mathbf{w}} \quad (26)$$

The second term on the right-hand side of Eq. (21) is then obtained by differentiating Eq. (26) with respect to the ensemble weights [see Eq. (22)]. Turning to the first term on the right-hand side of Eq. (21), the simplest way to obtain a density-functional expression is to connect the individual  $\overline{\text{SD}}$  correlation energy to the first (SD) one, as follows:

$$\begin{aligned} E_{c,J}^{\mathbf{w},\overline{\text{SD}}}[n^{\mathbf{w}}] &= E_{c,J}^{\mathbf{w},\text{SD}}[n^{\mathbf{w}}] \\ &+ 2 \sum_{I=1}^M \sum_{K \neq J}^M (\delta_{IK} - \mathbf{w}_I) \mathbf{w}_K \left\langle \Phi_K^{\mathbf{w}} \left| \hat{T} + \hat{W}_{ee} \right| \frac{\partial \Phi_K^{\mathbf{w}}}{\partial \mathbf{w}_I} \right\rangle, \end{aligned} \quad (27)$$

thus leading to the final expression

$$\begin{aligned} E_{c,J}^{\mathbf{w},\overline{\text{SD}}}[n^{\mathbf{w}}] &= E_{c,J}^{\mathbf{w},\text{SD}}[n^{\mathbf{w}}] \\ &+ \sum_{K \neq J}^M \sum_{I=1}^M \mathbf{w}_K (\delta_{IK} - \mathbf{w}_I) \frac{\partial f_K^{\mathbf{w}}[n^{\mathbf{w}}]}{\partial \mathbf{w}_I}. \end{aligned} \quad (28)$$

#### D. $\overline{\text{DD}}$ ensemble correlation energy

According to Eq. (21), the weighted sum  $E_c^{\mathbf{w},\overline{\text{SD}}}[n^{\mathbf{w}}]$  of the  $\overline{\text{SD}}$  correlation energies reads

$$\begin{aligned} E_c^{\mathbf{w},\overline{\text{SD}}}[n^{\mathbf{w}}] &= \sum_{J=0}^M \mathbf{w}_J E_{c,J}^{\mathbf{w},\overline{\text{SD}}}[n^{\mathbf{w}}] \\ &= \sum_{J=0}^M \mathbf{w}_J \left( \langle \Psi_J | \hat{T} + \hat{W}_{ee} | \Psi_J \rangle - f_J^{\mathbf{w}}[n^{\mathbf{w}}] \right) \\ &\quad - \sum_{J=0}^M \mathbf{w}_J^2 \sum_{I=1}^M (\delta_{IJ} - \mathbf{w}_I) \frac{\partial f_J^{\mathbf{w}}[n^{\mathbf{w}}]}{\partial \mathbf{w}_I}, \end{aligned} \quad (29)$$

or, equivalently,

$$E_c^{\mathbf{w},\overline{\text{SD}}}[n^{\mathbf{w}}] = E_c^{\mathbf{w}}[n^{\mathbf{w}}] - \sum_{J=0}^M \mathbf{w}_J^2 \sum_{I=1}^M (\delta_{IJ} - \mathbf{w}_I) \frac{\partial f_J^{\mathbf{w}}[n^{\mathbf{w}}]}{\partial \mathbf{w}_I}, \quad (30)$$

thus leading to the final expression

$$\begin{aligned} E_c^{\mathbf{w},\overline{\text{DD}}}[n^{\mathbf{w}}] &= E_c^{\mathbf{w}}[n^{\mathbf{w}}] - E_c^{\mathbf{w},\overline{\text{SD}}}[n^{\mathbf{w}}] \\ &= \sum_{J=0}^M \mathbf{w}_J^2 \sum_{I=1}^M (\delta_{IJ} - \mathbf{w}_I) \frac{\partial f_J^{\mathbf{w}}[n^{\mathbf{w}}]}{\partial \mathbf{w}_I}. \end{aligned} \quad (31)$$

## II. APPLICATION TO THE HUBBARD DIMER

### A. Densities and functionals

For simplicity, we focus on the weakly asymmetric and strongly correlated regime  $\Delta v_{\text{ext}}/t \ll t/U \ll 1$ . In this case, the ground state remains essentially symmetric [5], i.e.  $n_{\Psi_0} \approx 1$ , and the density of the first (singlet) excited state varies through first order in  $\Delta v_{\text{ext}}/t$  as  $n_{\Psi_1} \approx 1 + [(U\Delta v_{\text{ext}})/(2t^2)]$  [4]. In the following we use the compact notation  $n_{\Psi_1} \approx 1 + \eta$ , where  $\eta = U\Delta v_{\text{ext}}/(2t^2) \ll 1$ . As a result, the biensemble density reads

$$n^{\mathbf{w}} \approx 1 + \mathbf{w}\eta, \quad (32)$$

where  $\mathbf{w} \equiv \mathbf{w}_1$ . The KS excited state is always symmetric ( $n_{\Phi_1} = 1$ ), even when the true interacting system is not [5]. Therefore, the KS ground-state density equals  $n_{\Phi_0} = (n^{\mathbf{w}} - \mathbf{w})/(1 - \mathbf{w})$ , thus leading to

$$n_{\Phi_0} \approx 1 + \frac{\mathbf{w}\eta}{(1 - \mathbf{w})}, \quad (33)$$

and the following expression for the two-weight ensemble KS density:

$$n^{\xi, \mathbf{w}} \approx 1 + \frac{(1 - \xi)\mathbf{w}\eta}{(1 - \mathbf{w})}. \quad (34)$$

As shown in Ref. [4], in the strongly correlated regime, the ensemble correlation functional reads, for  $|n - 1| \leq \mathbf{w}$ , as follows:

$$E_c^{\mathbf{w}}(n) \approx -\frac{U}{2} \left[ (1 - \mathbf{w}) - \frac{(3\mathbf{w} - 1)(n - 1)^2}{(1 - \mathbf{w})^2} \right]. \quad (35)$$

### B. First (so-called SD/DD) decomposition

The SD/DD decomposition of each individual correlation energy is obtained from the following general expressions:

$$E_{c,J}^{\mathbf{w},\text{SD}}[n^{\mathbf{w}}] = E_c^{\mathbf{w}}[n^{\mathbf{w}}] + \sum_{I=1}^M (\delta_{IJ} - \mathbf{w}_I) \frac{\partial E_c^{\mathbf{w}}[n^{\mathbf{w}}]}{\partial \mathbf{w}_I} \quad (36)$$

and

$$E_{c,J}^{\mathbf{w},\text{DD}}[n^{\mathbf{w}}] = - \sum_{I=1}^M (\delta_{IJ} - \mathbf{w}_I) \frac{\partial E_c^{\xi}[n^{\xi, \mathbf{w}}]}{\partial \mathbf{w}_I} \Big|_{\xi=\mathbf{w}}. \quad (37)$$

According to Eq. (35), we have

$$E_c^{\mathbf{w}}(n^{\mathbf{w}}) \approx -\frac{U}{2} \left[ (1 - \mathbf{w}) - \frac{(3\mathbf{w} - 1)\mathbf{w}^2\eta^2}{(1 - \mathbf{w})^2} \right] \quad (38)$$

and

$$E_c^{\xi}(n^{\xi, \mathbf{w}}) \approx -\frac{U}{2} \left[ (1 - \xi) - \frac{(3\xi - 1)\mathbf{w}^2\eta^2}{(1 - \mathbf{w})^2} \right], \quad (39)$$

thus leading to the following derivative expressions,

$$\frac{dE_c^{\mathbf{w}}(n^{\mathbf{w}})}{d\mathbf{w}} \approx \frac{U}{2} \left[ 1 - \frac{\mathbf{w}(3\mathbf{w}^2 - 9\mathbf{w} + 2)\eta^2}{(1 - \mathbf{w})^3} \right] \quad (40)$$

and

$$\frac{\partial E_c^{\xi}(n^{\xi, \mathbf{w}})}{\partial \mathbf{w}} \approx U \frac{(3\xi - 1)\eta^2\mathbf{w}}{(1 - \mathbf{w})^3}, \quad (41)$$

from which we obtain

$$\begin{aligned} E_{c,J=0}^{\mathbf{w},\text{SD}}(n^{\mathbf{w}}) &= E_c^{\mathbf{w}}(n^{\mathbf{w}}) - \mathbf{w} \frac{dE_c^{\mathbf{w}}(n^{\mathbf{w}})}{d\mathbf{w}} \\ &\approx -\frac{U}{2} \left[ 1 - \frac{\mathbf{w}^2(1 - 5\mathbf{w})\eta^2}{(1 - \mathbf{w})^3} \right] \end{aligned} \quad (42)$$

and

$$\begin{aligned} E_{c,J=0}^{\mathbf{w},\text{DD}}(n^{\mathbf{w}}) &= \mathbf{w} \frac{\partial E_c^{\xi}(n^{\xi, \mathbf{w}})}{\partial \mathbf{w}} \Big|_{\xi=\mathbf{w}} \\ &\approx U \frac{(3\mathbf{w} - 1)\eta^2\mathbf{w}^2}{(1 - \mathbf{w})^3}. \end{aligned} \quad (43)$$

Finally, we deduce the excited-state SD/DD decomposition from the ground-state one as follows:

$$\begin{aligned} E_{c,J=1}^{\mathbf{w},\text{SD}}(n^{\mathbf{w}}) &= \frac{1}{\mathbf{w}} \left[ E_c^{\mathbf{w}}(n^{\mathbf{w}}) - (1 - \mathbf{w}) E_{c,J=0}^{\mathbf{w},\text{SD}}(n^{\mathbf{w}}) \right] \\ &\approx U\eta^2 \frac{\mathbf{w}(4\mathbf{w} - 1)}{(1 - \mathbf{w})^2} \end{aligned} \quad (44)$$

and

$$\begin{aligned} E_{c,J=1}^{\mathbf{w},\text{DD}}(n^{\mathbf{w}}) &= -\frac{(1 - \mathbf{w})}{\mathbf{w}} E_{c,J=0}^{\mathbf{w},\text{DD}}(n^{\mathbf{w}}) \\ &\approx -U\eta^2 \frac{(3\mathbf{w} - 1)\mathbf{w}}{(1 - \mathbf{w})^2}. \end{aligned} \quad (45)$$

### C. Second (so-called $\overline{\text{SD}}/\overline{\text{DD}}$ ) decomposition

In the regime under study, the exchange-only GOK functional can be simplified as follows [4, 5]:

$$\begin{aligned} f^{\xi}(n) &= -2t\sqrt{(1 - \xi)^2 - (1 - n)^2} \\ &\quad + \frac{U}{2} \left[ 1 + \xi - \frac{(3\xi - 1)(1 - n)^2}{(1 - \xi)^2} \right] \\ &\stackrel{|1-n| \ll 1}{\approx} -2t(1 - \xi) \left[ 1 - \frac{(1 - n)^2}{2(1 - \xi)^2} \right] \\ &\quad + \frac{U}{2} \left[ 1 + \xi - \frac{(3\xi - 1)(1 - n)^2}{(1 - \xi)^2} \right] \\ &\stackrel{\frac{t}{U} \ll 1}{\approx} \frac{U}{2} \left[ 1 + \xi - \frac{(3\xi - 1)(1 - n)^2}{(1 - \xi)^2} \right], \end{aligned} \quad (46)$$

thus leading to

$$f^{\mathbf{w}}(n^{\mathbf{w}}) \approx \frac{U}{2} \left[ 1 + \mathbf{w} - \frac{(3\mathbf{w} - 1)\mathbf{w}^2\eta^2}{(1 - \mathbf{w})^2} \right], \quad (47)$$

$$f^{\xi}(n^{\xi, \mathbf{w}}) \approx \frac{U}{2} \left[ 1 + \xi - \frac{(3\xi - 1)\mathbf{w}^2\eta^2}{(1 - \mathbf{w})^2} \right], \quad (48)$$

and

$$\frac{\partial f^{\xi}(n^{\xi, \mathbf{w}})}{\partial \xi} \approx \frac{U}{2} \left[ 1 - \frac{3\mathbf{w}^2\eta^2}{(1 - \mathbf{w})^2} \right]. \quad (49)$$

From the general expression in Eq. (26) we deduce the individual components of the exchange-only GOK energy,

$$f_{J=0}^{\mathbf{w}}(n^{\mathbf{w}}) = f^{\mathbf{w}}(n^{\mathbf{w}}) - \mathbf{w} \frac{\partial f^{\xi}(n^{\xi, \mathbf{w}})}{\partial \xi} \Big|_{\xi=\mathbf{w}} \quad (50)$$

$$\approx \frac{U}{2} \left[ 1 + \frac{\mathbf{w}^2\eta^2}{(1 - \mathbf{w})^2} \right], \quad (51)$$

and

$$f_{J=1}^{\mathbf{w}}(n^{\mathbf{w}}) = f^{\mathbf{w}}(n^{\mathbf{w}}) + (1 - \mathbf{w}) \frac{\partial f^{\xi}(n^{\xi, \mathbf{w}})}{\partial \xi} \Big|_{\xi=\mathbf{w}} \quad (52)$$

$$\approx U \left[ 1 - \frac{\mathbf{w}^2\eta^2}{(1 - \mathbf{w})^2} \right], \quad (53)$$

thus leading to the following derivative expressions:

$$\frac{\partial f_{K=0}^{\mathbf{w}}(n^{\mathbf{w}})}{\partial \mathbf{w}} \approx U\eta^2 \frac{\mathbf{w}}{(1-\mathbf{w})^3}, \quad (54)$$

$$\frac{\partial f_{K=1}^{\mathbf{w}}(n^{\mathbf{w}})}{\partial \mathbf{w}} \approx -U\eta^2 \frac{2\mathbf{w}}{(1-\mathbf{w})^3}. \quad (55)$$

The  $\overline{\text{SD}}/\overline{\text{DD}}$  decomposition can now be deduced from the SD/DD one by using the general expression in Eq. (28) and the fact that both decompositions give the same individual correlation energy, i.e.

$$E_{c,J}^{\mathbf{w},\overline{\text{DD}}}[n^{\mathbf{w}}] = E_{c,J}^{\mathbf{w},\text{DD}}[n^{\mathbf{w}}] - \left( E_{c,J}^{\mathbf{w},\overline{\text{SD}}}[n^{\mathbf{w}}] - E_{c,J}^{\mathbf{w},\text{SD}}[n^{\mathbf{w}}] \right), \quad (56)$$

thus leading to

$$\begin{aligned} E_{c,J=0}^{\mathbf{w},\overline{\text{SD}}}(n^{\mathbf{w}}) &= E_{c,J=0}^{\mathbf{w},\text{SD}}(n^{\mathbf{w}}) - \mathbf{w}^2 \frac{\partial f_{K=1}^{\mathbf{w}}(n^{\mathbf{w}})}{\partial \mathbf{w}} \\ &\approx -\frac{U}{2} \left[ 1 - \frac{\mathbf{w}^2 \eta^2}{(1-\mathbf{w})^2} \right], \end{aligned} \quad (57)$$

$$E_{c,J=0}^{\mathbf{w},\overline{\text{DD}}}(n^{\mathbf{w}}) \approx -U\eta^2 \frac{\mathbf{w}^2}{(1-\mathbf{w})^2}, \quad (58)$$

$$\begin{aligned} E_{c,J=1}^{\mathbf{w},\overline{\text{SD}}}(n^{\mathbf{w}}) &= E_{c,J=1}^{\mathbf{w},\text{SD}}(n^{\mathbf{w}}) + (1-\mathbf{w})^2 \frac{\partial f_{K=0}^{\mathbf{w}}(n^{\mathbf{w}})}{\partial \mathbf{w}} \\ &\approx U\eta^2 \frac{3\mathbf{w}^2}{(1-\mathbf{w})^2}, \end{aligned} \quad (59)$$

and

$$E_{c,J=1}^{\mathbf{w},\overline{\text{DD}}}(n^{\mathbf{w}}) \approx -U\eta^2 \frac{2\mathbf{w}^2}{(1-\mathbf{w})^2}. \quad (60)$$

The  $\overline{\text{SD}}/\overline{\text{DD}}$  decomposition is plotted in Fig. 1 for the excited state and compared with the SD/DD one.

We finally obtain the  $\overline{\text{SD}}/\overline{\text{DD}}$  decomposition of the ensemble correlation energy as follows:

$$\begin{aligned} E_c^{\mathbf{w},\overline{\text{SD}}}(n^{\mathbf{w}}) &= (1-\mathbf{w})E_{c,J=0}^{\mathbf{w},\overline{\text{SD}}}(n^{\mathbf{w}}) + \mathbf{w}E_{c,J=1}^{\mathbf{w},\overline{\text{SD}}}(n^{\mathbf{w}}) \\ &\approx -\frac{U(1-\mathbf{w})}{2} + U\eta^2 \frac{\mathbf{w}^2(1+5\mathbf{w})}{2(1-\mathbf{w})^2}, \end{aligned} \quad (61)$$

and

$$\begin{aligned} E_c^{\mathbf{w},\overline{\text{DD}}}(n^{\mathbf{w}}) &= (1-\mathbf{w})E_{c,J=0}^{\mathbf{w},\overline{\text{DD}}}(n^{\mathbf{w}}) + \mathbf{w}E_{c,J=1}^{\mathbf{w},\overline{\text{DD}}}(n^{\mathbf{w}}) \\ &\approx -U\eta^2 \frac{\mathbf{w}^2(1+\mathbf{w})}{(1-\mathbf{w})^2}. \end{aligned} \quad (62)$$

#### D. Approximate ensemble correlation energies

Within the GSc- $\overline{\text{SD}}$  approximation, the  $\overline{\text{SD}}$  part of the ensemble correlation energy is simplified as follows:

$$E_c^{\mathbf{w},\overline{\text{SD}}}(n^{\mathbf{w}}) \stackrel{\text{GSc-}\overline{\text{SD}}}{\approx} (1-\mathbf{w}) E_c(n_{\Psi_0}), \quad (63)$$

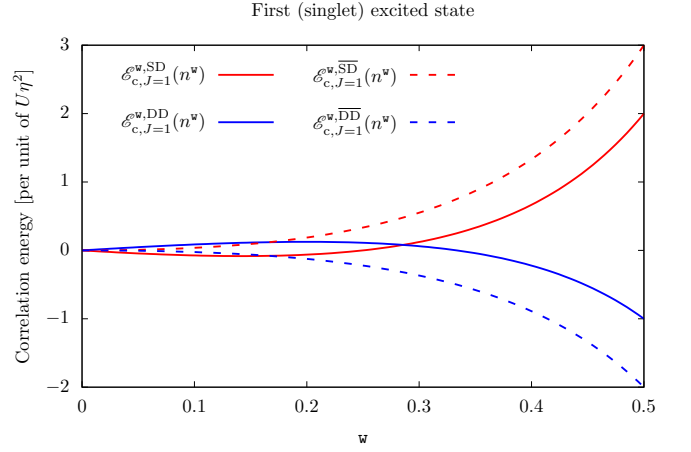

Figure 1: Comparison of SD/DD and  $\overline{\text{SD}}/\overline{\text{DD}}$  decompositions for the first (singlet) excited state of the weakly asymmetric and strongly correlated Hubbard dimer.

where  $n_{\Psi_0} \approx 1$  and

$$E_c(n) = E_c^{\mathbf{w}=0}(n) \approx -\frac{U}{2} [1 + (n-1)^2], \quad (64)$$

thus leading to

$$E_c^{\mathbf{w},\overline{\text{SD}}}(n^{\mathbf{w}}) \stackrel{\text{GSc-}\overline{\text{SD}}}{\approx} -\frac{U}{2} (1-\mathbf{w}). \quad (65)$$

In the regime under study, the GSc- $\overline{\text{DD}}$  approximation consists in simplifying the exchange-only GOK functional as follows [see Eq. (46)]:

$$f^\xi(n) \stackrel{\text{GSc-}\overline{\text{DD}}}{\approx} E_{\text{Hx}}(n) = \frac{U}{2} (1 + (1-n)^2), \quad (66)$$

thus leading to

$$f^\xi(n^{\xi,\mathbf{w}}) \stackrel{\text{GSc-}\overline{\text{DD}}}{\approx} \frac{U}{2} \left[ 1 + \frac{(1-\xi)^2 \mathbf{w}^2 \eta^2}{(1-\mathbf{w})^2} \right], \quad (67)$$

$$\frac{\partial f^\xi(n^{\xi,\mathbf{w}})}{\partial \xi} \stackrel{\text{GSc-}\overline{\text{DD}}}{\approx} -U\eta^2 \frac{\mathbf{w}^2(1-\xi)}{(1-\mathbf{w})^2}, \quad (68)$$

$$f^{\mathbf{w}}(n^{\mathbf{w}}) \stackrel{\text{GSc-}\overline{\text{DD}}}{\approx} \frac{U}{2} [1 + \mathbf{w}^2 \eta^2], \quad (69)$$

and [see Eqs. (50) and (52)]

$$f_{J=0}^{\mathbf{w}}(n^{\mathbf{w}}) \stackrel{\text{GSc-}\overline{\text{DD}}}{\approx} \frac{U}{2} \left[ 1 + \frac{\mathbf{w}^2 \eta^2 (1+\mathbf{w})}{1-\mathbf{w}} \right], \quad (70)$$

$$\frac{\partial f_{J=0}^{\mathbf{w}}(n^{\mathbf{w}})}{\partial \mathbf{w}} \stackrel{\text{GSc-}\overline{\text{DD}}}{\approx} U\eta^2 \frac{\mathbf{w}[1+\mathbf{w}(1-\mathbf{w})]}{(1-\mathbf{w})^2}, \quad (71)$$

$$f_{J=1}^{\mathbf{w}}(n^{\mathbf{w}}) \stackrel{\text{GSc-}\overline{\text{DD}}}{\approx} \frac{U}{2} [1 - \mathbf{w}^2 \eta^2], \quad (72)$$

$$\frac{\partial f_{J=1}^{\mathbf{w}}(n^{\mathbf{w}})}{\partial \mathbf{w}} \stackrel{\text{GSx-}\overline{\text{DD}}}{\approx} -U\eta^2 \mathbf{w}. \quad (73)$$

From the general and exact expression,

$$E_c^{\mathbf{w}, \overline{\text{DD}}}[n^{\mathbf{w}}] = \sum_{J=0}^M \mathbf{w}_J^2 \sum_{I=1}^M (\delta_{IJ} - \mathbf{w}_I) \frac{\partial f_J^{\mathbf{w}}[n^{\mathbf{w}}]}{\partial \mathbf{w}_I}, \quad (74)$$

we finally obtain

$$E_c^{\mathbf{w}, \overline{\text{DD}}}(n^{\mathbf{w}}) = -\mathbf{w}(1-\mathbf{w})^2 \frac{\partial f_{J=0}^{\mathbf{w}}(n^{\mathbf{w}})}{\partial \mathbf{w}} + \mathbf{w}^2(1-\mathbf{w}) \frac{\partial f_{J=1}^{\mathbf{w}}(n^{\mathbf{w}})}{\partial \mathbf{w}} \quad (75)$$

$$\stackrel{\text{GSx-}\overline{\text{DD}}}{\approx} -U\eta^2 \mathbf{w}^2 [1 + 2\mathbf{w}(1-\mathbf{w})]. \quad (76)$$

Both GSc- $\overline{\text{SD}}$  and GSx- $\overline{\text{DD}}$  contributions to the ensemble correlation energy are plotted in Fig. 2. We observe that, beyond the leading (zeroth) order in  $\eta$  [see also Eqs. (61) and (62)], the exact  $\overline{\text{SD}}$  and  $\overline{\text{DD}}$  corrections have opposite sign [see the “exact  $\overline{\text{SD}}$  only” and “GSc- $\overline{\text{SD}}$ +exact  $\overline{\text{DD}}$ ” curves] so that the total (second-order-in- $\eta$ ) correction barely vary with the ensemble weight  $\mathbf{w}$ . A slight increase can be seen when approaching the equiensemble limit. This feature is (not perfectly but) relatively

well reproduced when combining the GSc- $\overline{\text{SD}}$  and GSx- $\overline{\text{DD}}$  approximations. Combining GSc- $\overline{\text{SD}}$  with the exact  $\overline{\text{DD}}$  correction leads to a substantial overestimation of the correlation energy. In summary, error cancellations can occur when combining  $\overline{\text{SD}}$  and  $\overline{\text{DD}}$  ensemble density-functional approximations. It is an important fact on which we may rely for turning the theory into an accurate computational method.

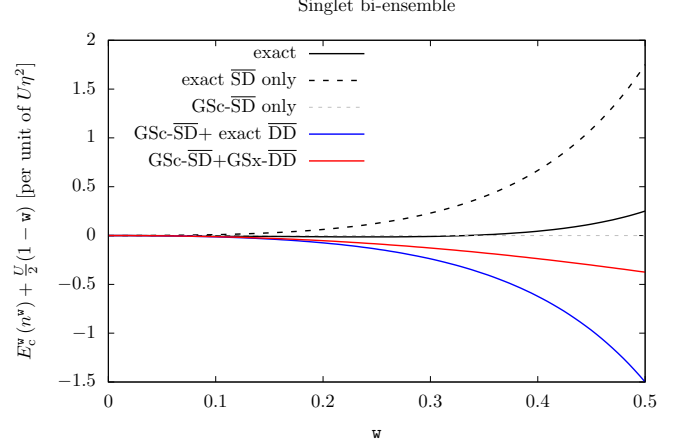

Figure 2: Exact and approximate  $\overline{\text{SD}}/\overline{\text{DD}}$  decompositions of the ensemble correlation energy in the weakly asymmetric and strongly correlated Hubbard dimer.

<sup>1</sup> M. Casida and M. Huix-Rotllant, *Annu. Rev. Phys. Chem.* **63**, 287 (2012).

<sup>2</sup> M. Filatov, F. Liu, and T. J. Martinez, *J. Chem. Phys.* **147**, 034113 (2017).

<sup>3</sup> B. Senjean, S. Knecht, H. J. Aa. Jensen, and E. Fromager, *Phys. Rev. A* **92**, 012518 (2015).

<sup>4</sup> K. Deur, L. Mazouin, B. Senjean, and E. Fromager, *Eur. Phys. J. B* **91**, 162 (2018).

<sup>5</sup> K. Deur, L. Mazouin, and E. Fromager, *Phys. Rev. B* **95**, 035120 (2017).
